# Supplementary material for: Selective Classification Under Distribution Shifts
Source: arXiv:2405.05160 source file (2024-11-27)
Supplement: Supplementary file 1 [file SAT-Details.tex]

\section{Self-adaptive-training reproduction details.}
\label{App: SAT training details}

Briefly speaking, we strictly follows the original training setups for the selective classification application stated in Section 4 and Appendix A.4 from \citet{huang2022self}, except that we did not use the VGG network but a ResNet34. Some important key points to mention are:
\begin{itemize}
    \item Introducing an extra logit (denoted by $f(\mb x)_c$) to predict the abstention score, and treat the training process as a $(C+1)$-class classification task, where $C=10$ for CIFAR-10 dataset.
    \item Optimizing the classifer with loss:
    \begin{equation}
        \ell(f) = -\frac{1}{m} \sum_i [\mb t_{i, y_i} \log \mb p_{i, y_i} + (1 - \mb t_{i, y_i}) \log \mb p_{i, c}]~\text{,}
    \end{equation}
    where $y_i$ is the index of non-zero element in the one-hot true label vector $\mb y_i$ corresponding to sample $\mb x_i$, $i$ is the sample index, $\mb t_i$ is the exponential moving average soft label vector defined in Alg. 1 and $\mb p_i$ is the model output $f(\mb x_i)$ after softmax normalization.
    \item The network is optimized using SGD with initial learning rate $0.1$, momentum $0.9$, weight decay $0.0005$, batch size $128$ and total training epoch is $300$. The learning rate decays by a factor of $0.5$ every $25$ epoch.
    \item Choice of hyper-parameters: $E_s = 0$ --- estimating the soft label by moving average staring at epoch $0$; $\alpha=0.99$ --- the exponetial decay rate.
\end{itemize}
