# Supplementary material for: Selective Classification Under Distribution Shifts
Source: arXiv:2405.05160 source file (2024-11-27)
Supplement: Supplementary file 5 [file AURC_computation.tex]

\section{AURC-$\alpha$ and AURC-$\beta$}
\label{App: Partial AURC formulas}
