# Supplementary material for: Selective Classification Under Distribution Shifts
Source: arXiv:2405.05160 source file (2024-11-27)
Supplement: Supplementary file 6 [file ImageNet-Exp.tex]

\section{Additional Experiment Results --- ImageNet}
\label{App: ImageNet Exp}

\subsection{RC Curves}
