# Supplementary material for: Selective Classification Under Distribution Shifts
Source: arXiv:2405.05160 source file (2024-11-27)
Supplement: Supplementary file 7 [file Cifar-RC-Curves-Lv5.tex]

\begin{figure}[ht]
\centering
\begingroup 
\begin{tabular}{c c c c}
\centering

\includegraphics[width=0.22\textwidth]{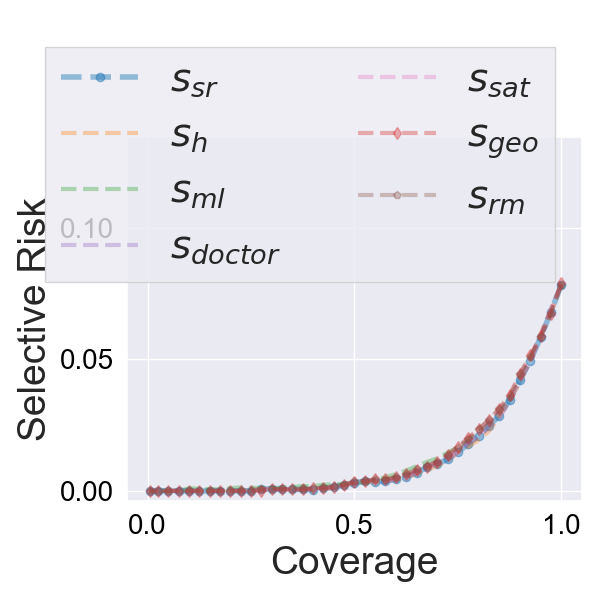}
&\includegraphics[width=0.22\textwidth]{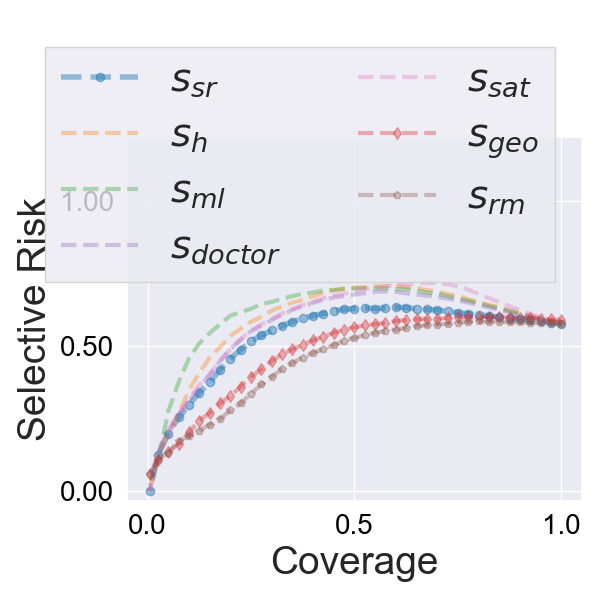}
&\includegraphics[width=0.22\textwidth]{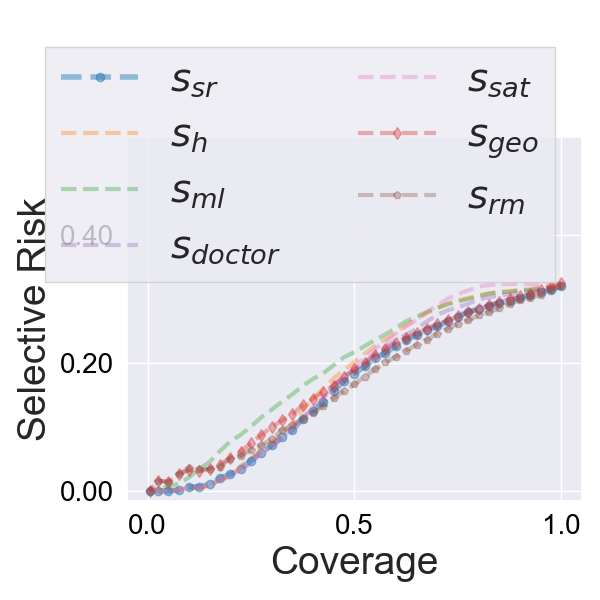}
&\includegraphics[width=0.22\textwidth]{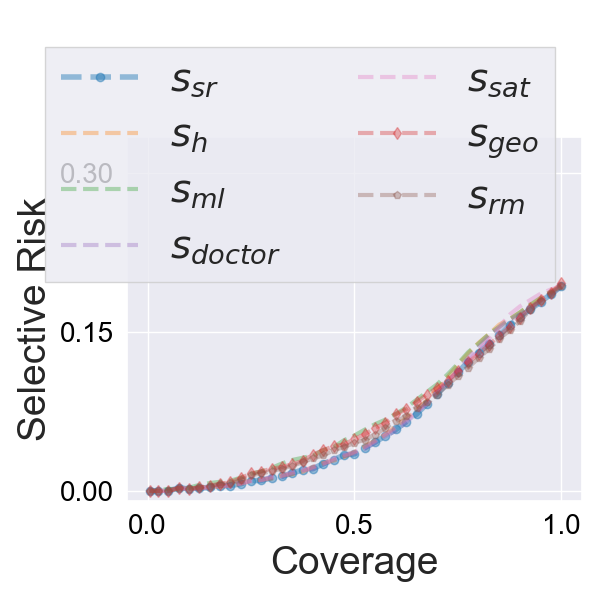}
\\
{\textbf{(a)} Brightness}
&{\textbf{(b)} Contrast}
&{\textbf{(c)} Defocus blur}
&{\textbf{(d)} Elastic}
\\
\includegraphics[width=0.22\textwidth]{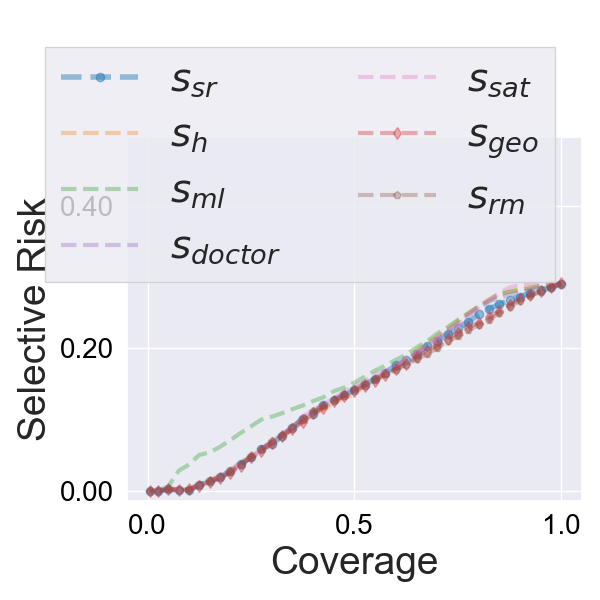}
&\includegraphics[width=0.22\textwidth]{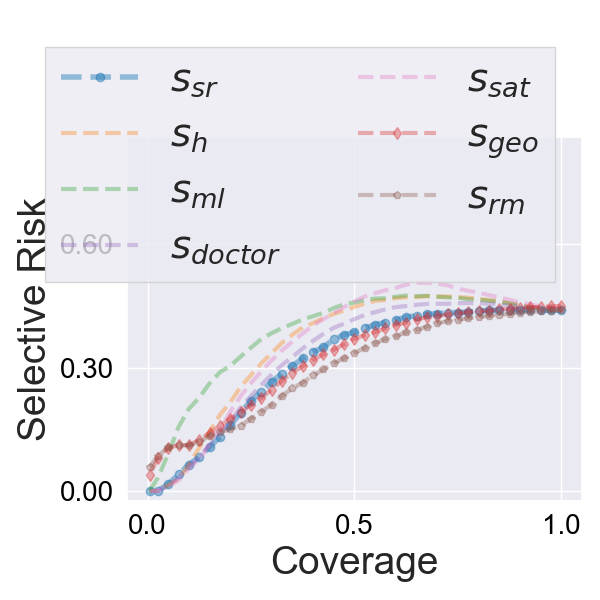}
&\includegraphics[width=0.22\textwidth]{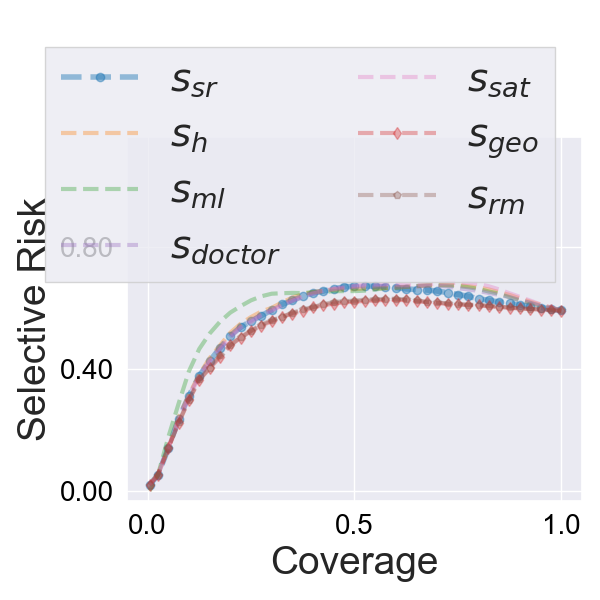}
&\includegraphics[width=0.22\textwidth]{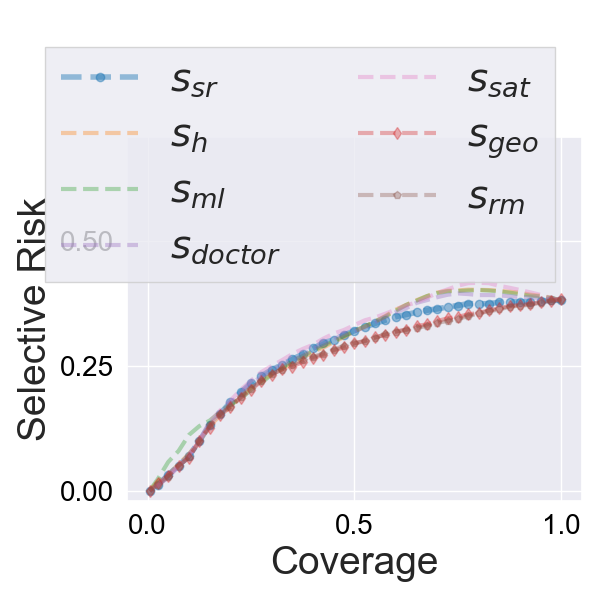}
\\
{\textbf{(e)} Frost}
&{\textbf{(f)} Gaussian blur}
&{\textbf{(g)} Gaussian noise}
&{\textbf{(h)} Glass blur}
\\
\includegraphics[width=0.22\textwidth]{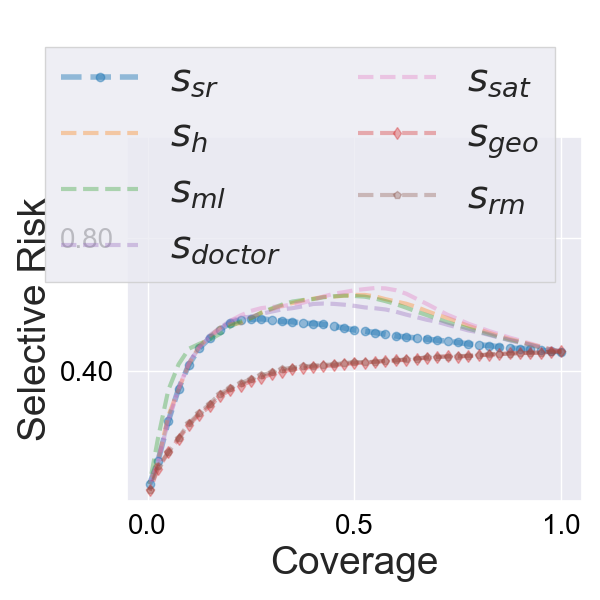}
&\includegraphics[width=0.22\textwidth]{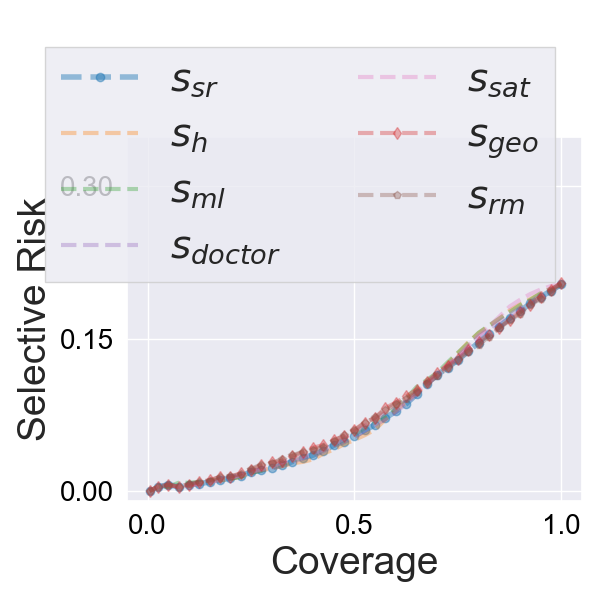}
&\includegraphics[width=0.22\textwidth]{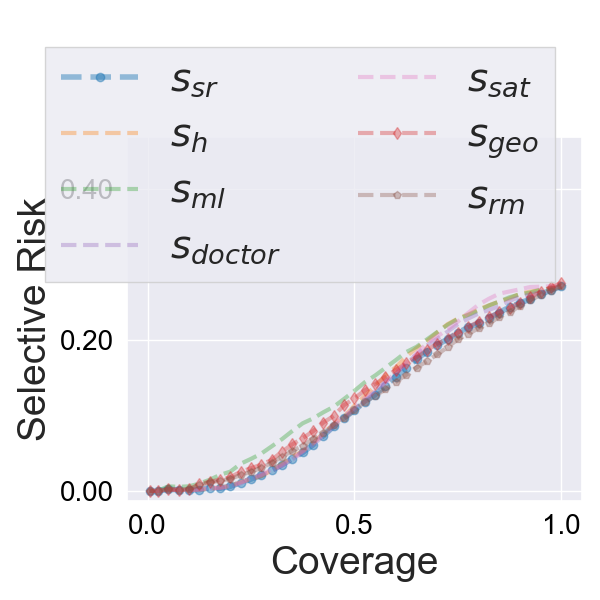}
&\includegraphics[width=0.22\textwidth]{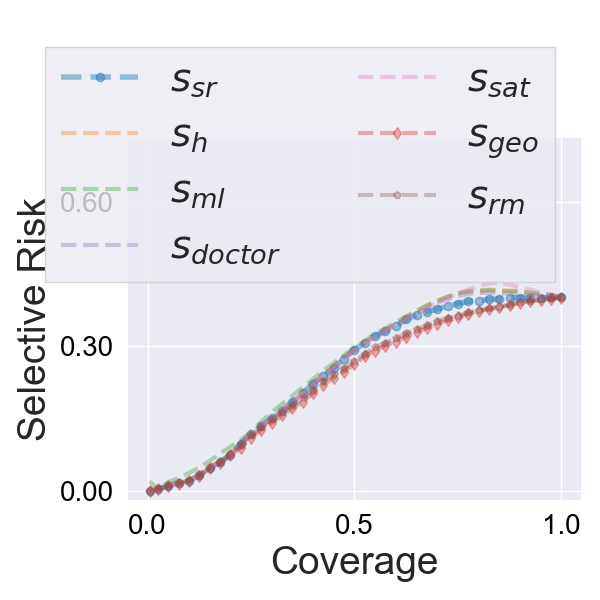}
\\
{\textbf{(i)} Impulse}
&{\textbf{(j)} JPEG}
&{\textbf{(k)} Motion blur}
&{\textbf{(l)} Pixelate}
\\
\includegraphics[width=0.22\textwidth]{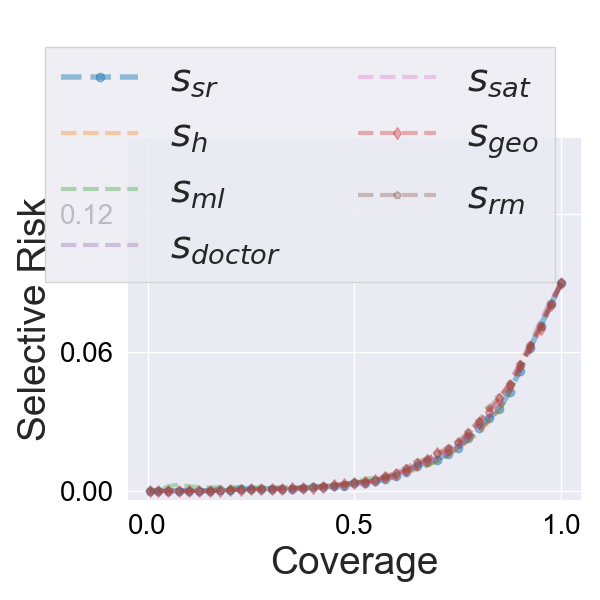}
&\includegraphics[width=0.22\textwidth]{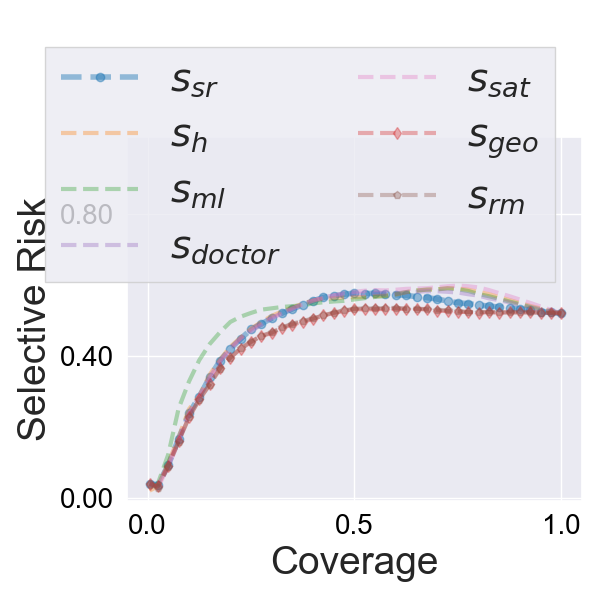}
&\includegraphics[width=0.22\textwidth]{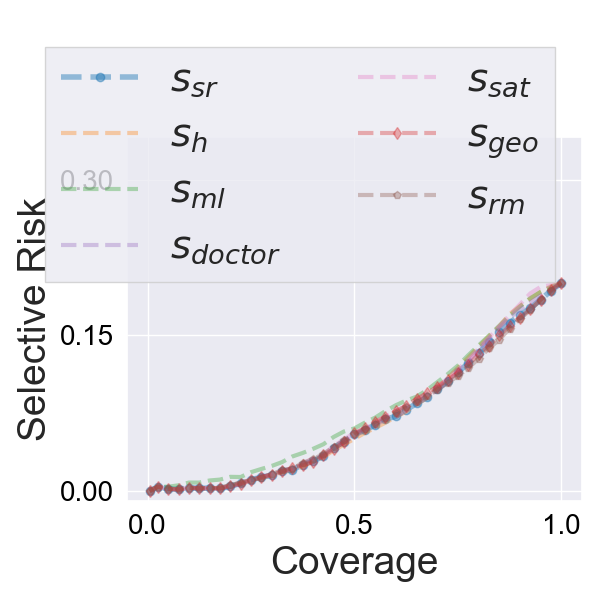}
&\includegraphics[width=0.22\textwidth]{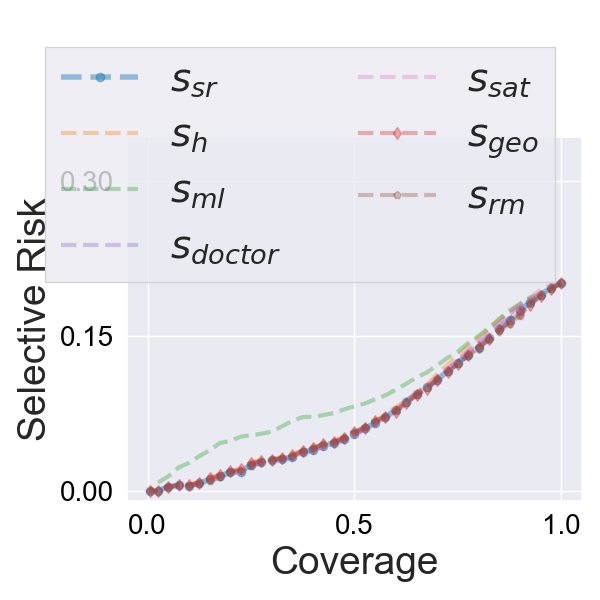}
\\
{\textbf{(m)} Saturate}
&{\textbf{(n)} Shot noise}
&{\textbf{(o)} Snow}
&{\textbf{(p)} Spatter}
\\
\includegraphics[width=0.22\textwidth]{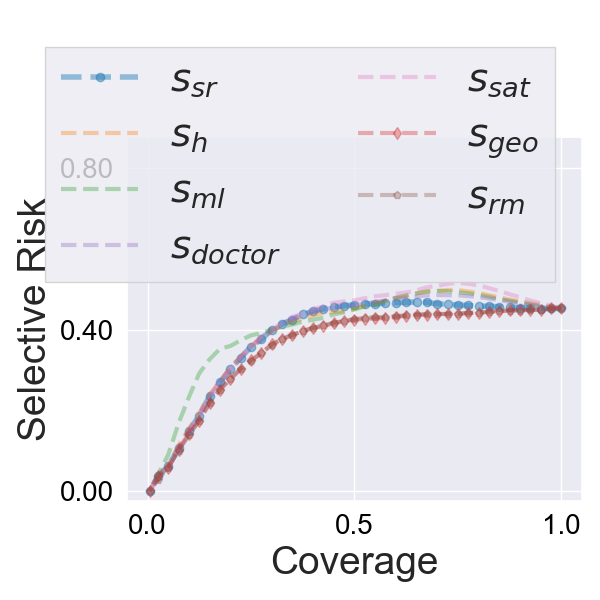}
&\includegraphics[width=0.22\textwidth]{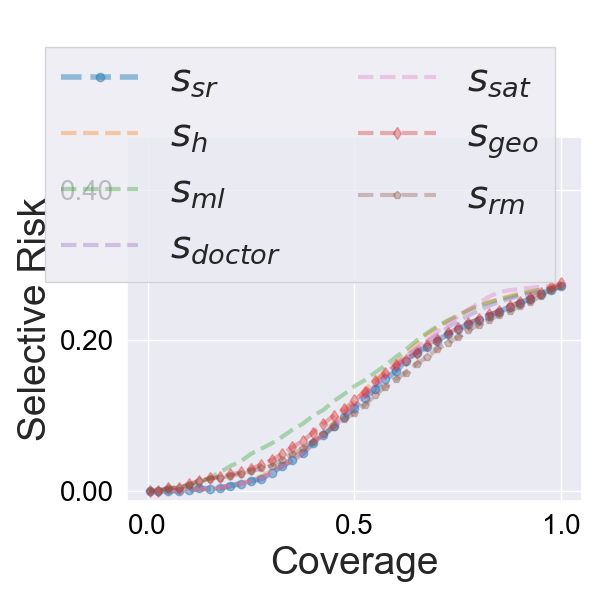}
&
&
\\
{\textbf{(q)} Speckle noise}
&{\textbf{(r)} Zoom blur}

\end{tabular}
\endgroup 
\caption{(Continuing \cref{Subsec: exp cifar10}) RC curves from the CIFAR-10-C dataset. All corruptions are at severity $5$. The difference in the performance of the confidence scores is more obvious when the classification performance at full coverage degrades substantially due to distribution shifts.}
\label{App Fig: Cifar10 RC curves Lv5}
\end{figure}
