# Supplementary material for: Selective Classification Under Distribution Shifts
Source: arXiv:2405.05160 source file (2024-11-27)
Supplement: Supplementary file 8 [file ImageNet-CoAtNet-RC-Lv1.tex]

\begin{figure}[ht]
\centering
\begingroup 
\begin{tabular}{c c c c}
\centering

\includegraphics[width=0.22\textwidth]{Figures/ImageNet/CoAtNet/brightness_1.png}
&\includegraphics[width=0.22\textwidth]{Figures/ImageNet/CoAtNet/contrast_1.png}
&\includegraphics[width=0.22\textwidth]{Figures/ImageNet/CoAtNet/defocus_blur_1.png}
&\includegraphics[width=0.22\textwidth]{Figures/ImageNet/CoAtNet/elastic_transform_1.png}
\\
{\textbf{(a)} Brightness}
&{\textbf{(b)} Contrast}
&{\textbf{(c)} Defocus blur}
&{\textbf{(d)} Elastic}
\\
\includegraphics[width=0.22\textwidth]{Figures/ImageNet/CoAtNet/frost_1.png}
&\includegraphics[width=0.22\textwidth]{Figures/ImageNet/CoAtNet/gaussian_blur_1.png}
&\includegraphics[width=0.22\textwidth]{Figures/ImageNet/CoAtNet/gaussian_noise_1.png}
&\includegraphics[width=0.22\textwidth]{Figures/ImageNet/CoAtNet/glass_blur_1.png}
\\
{\textbf{(e)} Frost}
&{\textbf{(f)} Gaussian blur}
&{\textbf{(g)} Gaussian noise}
&{\textbf{(h)} Glass blur}
\\
\includegraphics[width=0.22\textwidth]{Figures/ImageNet/CoAtNet/impulse_noise_1.png}
&\includegraphics[width=0.22\textwidth]{Figures/ImageNet/CoAtNet/jpeg_compression_1.png}
&\includegraphics[width=0.22\textwidth]{Figures/ImageNet/CoAtNet/motion_blur_1.png}
&\includegraphics[width=0.22\textwidth]{Figures/ImageNet/CoAtNet/pixelate_1.png}
\\
{\textbf{(i)} Impulse}
&{\textbf{(j)} JPEG}
&{\textbf{(k)} Motion blur}
&{\textbf{(l)} Pixelate}
\\
\includegraphics[width=0.22\textwidth]{Figures/ImageNet/CoAtNet/saturate_1.png}
&\includegraphics[width=0.22\textwidth]{Figures/ImageNet/CoAtNet/shot_noise_1.png}
&\includegraphics[width=0.22\textwidth]{Figures/ImageNet/CoAtNet/snow_1.png}
&\includegraphics[width=0.22\textwidth]{Figures/ImageNet/CoAtNet/spatter_1.png}
\\
{\textbf{(m)} Saturate}
&{\textbf{(n)} Shot noise}
&{\textbf{(o)} Snow}
&{\textbf{(p)} Spatter}
\\
\includegraphics[width=0.22\textwidth]{Figures/ImageNet/CoAtNet/speckle_noise_1.png}
&\includegraphics[width=0.22\textwidth]{Figures/ImageNet/CoAtNet/zoom_blur_1.png}
&\includegraphics[width=0.22\textwidth]{Figures/ImageNet/CoAtNet/ImageNet-Clean.png}
&
\\
{\textbf{(q)} Speckle noise}
&{\textbf{(r)} Zoom blur}
&{\textbf{(s)} IN (Clean)}

\end{tabular}
\endgroup 
\caption{(Continuing \cref{Subsec: ImageNet Experiments}) RC curves of different confidence scores achieved by the model \textbf{CoAtNet} on ImageNet-C (severity Lv.1) and IN (clean) images.}
\label{App Fig: ImageNet CoAtNet RC curve Lv1}
\end{figure}
