# Supplementary material for: Selective Classification Under Distribution Shifts
Source: arXiv:2405.05160 source file (2024-11-27)
Supplement: Supplementary file 13 [file ImageNet-ResNext-RC-Lv5.tex]

\begin{figure}[ht]
\centering
\begingroup 
\begin{tabular}{c c c c}
\centering

\includegraphics[width=0.22\textwidth]{Figures/ImageNet/ResNext/brightness_5.png}
&\includegraphics[width=0.22\textwidth]{Figures/ImageNet/ResNext/contrast_5.png}
&\includegraphics[width=0.22\textwidth]{Figures/ImageNet/ResNext/defocus_blur_5.png}
&\includegraphics[width=0.22\textwidth]{Figures/ImageNet/ResNext/elastic_transform_5.png}
\\
{\textbf{(a)} Brightness}
&{\textbf{(b)} Contrast}
&{\textbf{(c)} Defocus blur}
&{\textbf{(d)} Elastic}
\\
\includegraphics[width=0.22\textwidth]{Figures/ImageNet/ResNext/frost_5.png}
&\includegraphics[width=0.22\textwidth]{Figures/ImageNet/ResNext/gaussian_blur_5.png}
&\includegraphics[width=0.22\textwidth]{Figures/ImageNet/ResNext/gaussian_noise_5.png}
&\includegraphics[width=0.22\textwidth]{Figures/ImageNet/ResNext/glass_blur_5.png}
\\
{\textbf{(e)} Frost}
&{\textbf{(f)} Gaussian blur}
&{\textbf{(g)} Gaussian noise}
&{\textbf{(h)} Glass blur}
\\
\includegraphics[width=0.22\textwidth]{Figures/ImageNet/ResNext/impulse_noise_5.png}
&\includegraphics[width=0.22\textwidth]{Figures/ImageNet/ResNext/jpeg_compression_5.png}
&\includegraphics[width=0.22\textwidth]{Figures/ImageNet/ResNext/motion_blur_5.png}
&\includegraphics[width=0.22\textwidth]{Figures/ImageNet/ResNext/pixelate_5.png}
\\
{\textbf{(i)} Impulse}
&{\textbf{(j)} JPEG}
&{\textbf{(k)} Motion blur}
&{\textbf{(l)} Pixelate}
\\
\includegraphics[width=0.22\textwidth]{Figures/ImageNet/ResNext/saturate_5.png}
&\includegraphics[width=0.22\textwidth]{Figures/ImageNet/ResNext/shot_noise_5.png}
&\includegraphics[width=0.22\textwidth]{Figures/ImageNet/ResNext/snow_5.png}
&\includegraphics[width=0.22\textwidth]{Figures/ImageNet/ResNext/spatter_5.png}
\\
{\textbf{(m)} Saturate}
&{\textbf{(n)} Shot noise}
&{\textbf{(o)} Snow}
&{\textbf{(p)} Spatter}
\\
\includegraphics[width=0.22\textwidth]{Figures/ImageNet/ResNext/speckle_noise_5.png}
&\includegraphics[width=0.22\textwidth]{Figures/ImageNet/ResNext/zoom_blur_5.png}
&
&
\\
{\textbf{(q)} Speckle noise}
&{\textbf{(r)} Zoom blur}
&
&

\end{tabular}
\endgroup 
\caption{(Continuing \cref{Subsec: ImageNet Experiments}) RC curves of different confidence scores achieved by the model \textbf{ResNext} on ImageNet-C (severity Lv.5).}
\label{App Fig: ImageNet ResNext RC curve Lv5}
\end{figure}
